# Supplementary material for: Realization of Attractive Level Crossing via a Dissipative Mode
Source: arXiv:1907.06222 ancillary file (2019-07-16)
Supplement: Supplementary file 1 [file SM_V4.pdf]

# Supplementary Materials: Realization of Attractive Level Crossing via a Dissipative Mode

Weichao Yu (余伟超),[1,2] Jiongjie Wang,[1] H. Y. Yuan,[3] and Jiang Xiao (萧江)[1,4,*]

[1]Department of Physics and State Key Laboratory of Surface Physics, Fudan University, Shanghai 200433, China
[2]Institute for Materials Research, Tohoku University, Sendai 980-8577, Japan
[3]Department of Physics, Southern University of Science and Technology, Shenzhen 518055, Guangdong, China
[4]Institute for Nanoelectronics Devices and Quantum Computing, Fudan University, Shanghai 200433, China

## ATTRACTIVE COUPLING IN HARMONIC OSCILLATORS

Fig. S1 shows the spectrums of the two coupled oscillators for the cases of a reactive spring, disspative (velocity) coupling, and dissipative (absement) coupling, as shown in Fig. 1 in the main text.

For the absement coupling as in Fig. 1(a-3), where the two oscillators are coupled (with strength $\kappa_i$) to a third oscillator of frequency $\omega_0$ which subjects to dissipative friction characterized by $\eta_0$. The equation of motions for $x_{i=1,2}$ and $x_0$

$$\ddot{x}_i + \omega_i^2 x_i = -\eta_i \dot{x}_i + \kappa_i (x_0 - x_i), \tag{S1a}$$

$$\ddot{x}_0 + \omega_0^2 x_0 = -\eta_0 \dot{x}_0 + \kappa_0 (x_1 + x_2) \simeq 0. \tag{S1b}$$

The second equation approximately vanishes when $\omega_0 \simeq 0$ and the mass $m_0$ is very tiny such that its inertia can be neglected. In such a situation, the friction force is balanced with the spring forces from $m_1$ and $m_2$. By eliminating $x_0$ in the equations for $x_i$, we obtain

$$\ddot{x}_i + (\omega_i^2 + \kappa_i) x_i + \eta_i \dot{x}_i = \frac{\kappa_i \kappa_0}{\eta_0} \hat{T}_{-1} (x_1 + x_2), \tag{S2}$$

equivalent to Eq. (1) with the absement ($\hat{T}_{-1}$) coupling.

## DERIVATION OF THE EFFECTIVE 2-OSCILLATOR HAMILTONIAN

To eliminate the coupling terms with the third-party

$$\hat{H} = \begin{pmatrix} \omega_1 & \kappa_{12} & \kappa_{10} \\ \kappa_{12}^* & \omega_2 & \kappa_{20} \\ \kappa_{01} & \kappa_{02} & \omega_0 \end{pmatrix} \to \begin{pmatrix} \omega_1' & \kappa_{12}' & 0 \\ {\kappa_{12}'}^* & \omega_2' & 0 \\ 0 & 0 & \omega_0' \end{pmatrix}, \tag{S3}$$

we use Schrieffer-Wolff transformation [? ] to transform the effect of mode-0 to the coupling of mode-1 and mode-2 by defining the generator,

$$S = \sum_{i=1,2} \frac{\kappa_{0i}}{\omega_i - \omega_0} (a_i^\dagger a_0 - a_i a_0^\dagger). \tag{S4}$$

When $\kappa_{12} = 0$, it is straightforward to justify the identify $V + [S, H_0] = 0$, where

$$H_0 = \sum_{j=0,1,2} \hbar \omega_j \hat{a}_j^\dagger \hat{a}_j \quad \text{and} \quad V = \sum_{i<j} \kappa_{jk} \left( \hat{a}_j^\dagger \hat{a}_k + \hat{a}_k^\dagger \hat{a}_j \right) \tag{S5}$$

are the non-perturbative and perturbative components of the Hamiltonian, respectively. Then the effective Hamiltonian can be written as

$$H' = e^S H e^{-S} = H + [S, H] + \frac{1}{2}[S, [S, H]] + \cdots = H_0 + \frac{1}{2}[S, V] + O(\kappa_{0i}^3) = \sum_{j=0,1,2} \hbar \omega_j' \hat{a}_j^\dagger \hat{a}_j + \kappa_{12}' (\hat{a}_1^\dagger \hat{a}_2 + \hat{a}_1 \hat{a}_2^\dagger), \tag{S6}$$

where

$$\omega_i' = \omega_i + \frac{\kappa_{0i}^2}{\omega_i - \omega_0}, \quad \omega_0' = \omega_0 - \sum_{i=1,2} \frac{\kappa_{0i}^2}{\omega_i - \omega_0}, \quad \text{and} \quad \kappa_{12}' = \kappa_{12} + \frac{1}{2} \kappa_{01} \kappa_{02} \sum_{i=1,2} \frac{1}{\omega_i - \omega_0}, \tag{S7}$$

and the last expression is valid when $\kappa_{12} \ll \kappa_{01}, \kappa_{02}$.

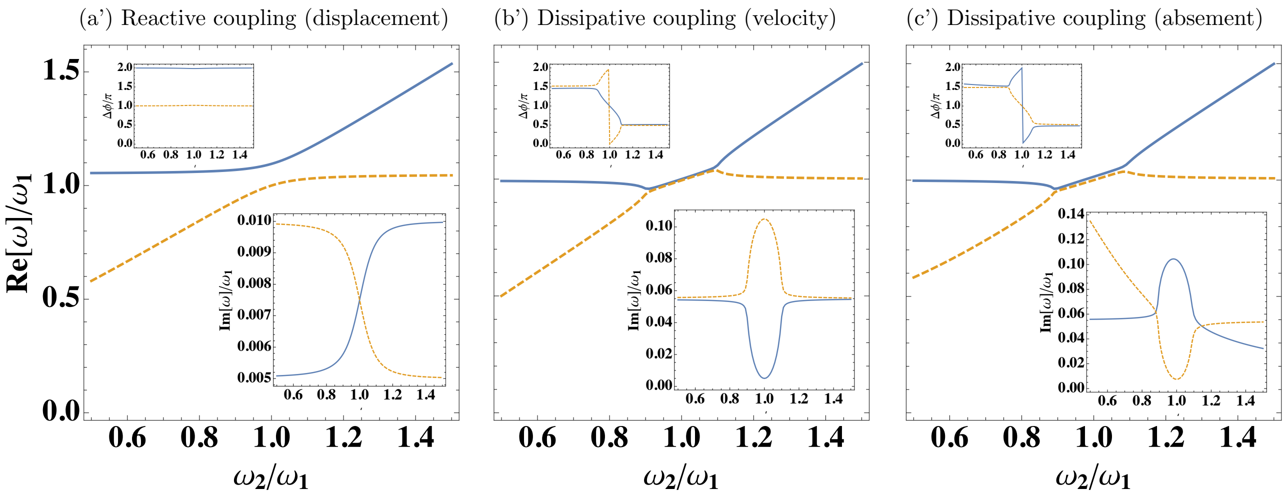


Figure S1. The level crossing behaviors for the three cases in Fig. 1. Insets: the imaginary part of eigenfrequencies (lower right) and the relative phase between the two mass (upper left). Parameters: $\kappa_i/\omega_1^2 = 0.1, \eta_1 = 0.01\omega_1, \eta_2 = 2\eta_1$ for (a) and $\eta_2 = \eta_1$ for (b,c).

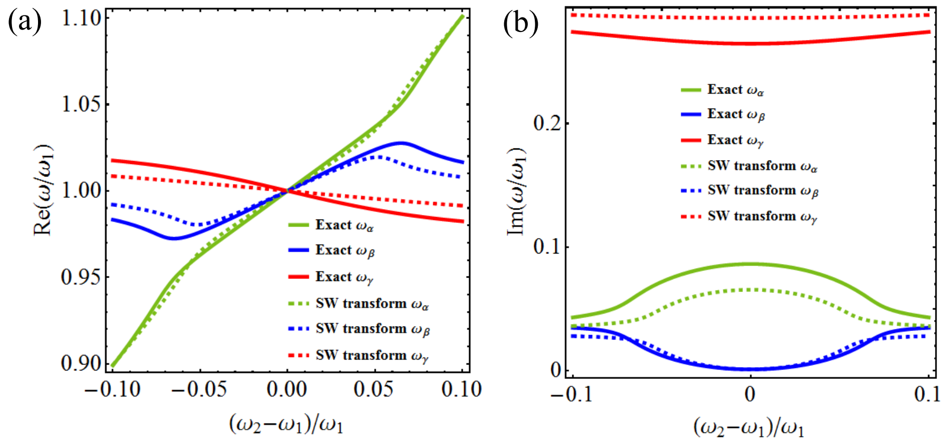


Figure S2. The eigen frequencies for the quantum model with the parameters same as Fig. 1(c). The solid and dashed lines represent the results of exact diagonalization of $\hat{H}$ in Eq. (4) and the reduced 2-mode Hamiltonian in Eq. (5), respectively. Inset: the imaginary part of the eigen frequencies.

## NUMERICAL SIMULATION

To verify the proposed model, we conduct finite-element simulation based on COMSOL Multiphysics [1]. In the spin cavitronics system, the spin dynamics is governed by the Landau-Lifshitz-Gilbert equation. When the external field is along $\hat{\mathbf{z}}$ direction, the magnetization $\mathbf{M} = \hat{\mathbf{z}} + \mathbf{m}$, and in the frequency domain, the small deviation $\mathbf{m}$ satisfies:

$$i\omega\mathbf{m} = \hat{\mathbf{z}} \times (\omega_M \mathbf{h} - \omega_H \mathbf{m} + i\alpha\omega\mathbf{m}) \tag{S8}$$

where $\omega_M = \gamma M_s$ with the saturated magnetization $M_s = 0.176\,\mathrm{T}$ [2], gyromagnetic ratio $\gamma = 28\,\mathrm{GHz/T}$, $\omega_H = \gamma H$ comes from the external field and $\alpha$ is the Gilbert damping $\alpha = 7.6 \times 10^{-5}$. Since Eq. (S8) can be represented in the form $\mathbf{m} = \chi\mathbf{h}$, and the equivalent permability of the YIG sphere is [3, 4]

$$\mu_{\mathrm{M}} = 1 + \chi = \begin{pmatrix} 1+u & -iv & 0 \\ iv & 1+u & 0 \\ 0 & 0 & 1 \end{pmatrix} \tag{S9}$$

where

$$u = \frac{(\omega_H - i\alpha\omega)\,\omega_M}{(\omega_H - i\alpha\omega)^2 - \omega^2}, \quad v = \frac{\omega\omega_M}{(\omega_H - i\alpha\omega)^2 - \omega^2} \tag{S10}$$

The electromagnetic wave in the cavity (including the YIG sphere) is governed by the Maxwell's equation,

$$\nabla \times \left[\mu(\mathbf{r})^{-1}\nabla \times \mathbf{E}\right] - k^2\varepsilon_r(\mathbf{r})\mathbf{E} = 0 \tag{S11}$$

with $k = \omega/c$ is the wave vector of light in vacuum. Here $\mu(\mathbf{r})$ and $\varepsilon_r(\mathbf{r})$ is the permeability and relative permittivity with $\mu(\mathbf{r}) = \mu_0(\mu_{\mathrm{M}})$ and $\varepsilon(\mathbf{r}) = 1(15)$ for the region outside (inside) the YIG sphere [3]. As shown in Fig. 2, two metal stripes with length 40mm and width 2.5mm are grown upon the dielectric substrate ($\varepsilon_r = 3.38$) with thickness 1.5mm. The distance between the central axis of two stripes is 3mm. The lower stripe is connected with input and output ports. By solving Eq. (S11) numerically in frequency domain, the full field distribution as well as the reflection (transmission) spectrum S11 (S21) can be calculated.

* Corresponding author: xiaojiang@fudan.edu.cn

[1] "COMSOL Multiphysics," .
[2] Y.-P. Wang, G.-Q. Zhang, D. Zhang, X.-Q. Luo, W. Xiong, S.-P. Wang, T.-F. Li, C.-M. Hu, and J. Q. You, Physical Review B **94**, 224410 (2016).
[3] B. Zare Rameshti and G. E. W. Bauer, Physical Review B **97**, 014419 (2018).
[4] Y. Cao, P. Yan, H. Huebl, S. T. B. Goennenwein, and G. E. W. Bauer, Physical Review B **91**, 094423 (2015).
